# Supplementary material for: StreamGS: Online Generalizable Gaussian Splatting Reconstruction for Unposed Image Streams
Source: arXiv:2503.06235 source file (2025-03-22)
Supplement: Supplementary file 1 [file X_suppl.tex]

\clearpage
\setcounter{page}{1}
\maketitlesupplementary

\section*{Implementation Details}
\label{sec:details}
We applied a consistent test protocol across all datasets. Each frame had a resolution of 224 × 224. For every video clip, we sampled 150 frames as context frames with a sampling ratio of 8. To-be-test frames were picked between the context frames uniformly, i.e., view interpolation. Noted that for training dataset RE10K, the selected frames are further from context frames than OOD datasets to make the comparison more clear, i.e., view extrapolation.

\section*{Robustness of Matching.} Matching head is frozen during the training. We use RANSAC to mitigate the impact of outliers' matches. Additionally, during the alignment, we assume camera motion is smooth and discard refinement results with excessively abrupt changes in translation and rotation. Although StreamGS could fail in texture-less regions, \textbf{it is more robust than baselines since its estimation would be much more accurate than raw prediction by DUSt3R}. An example in \cref{fig:robustsness} shows the robustness of adaptive refinement in texture-less region. 
% We would add a limitation discussion about it.

\begin{figure}[htbp]
    \centering
        \includegraphics[width=0.5\textwidth]{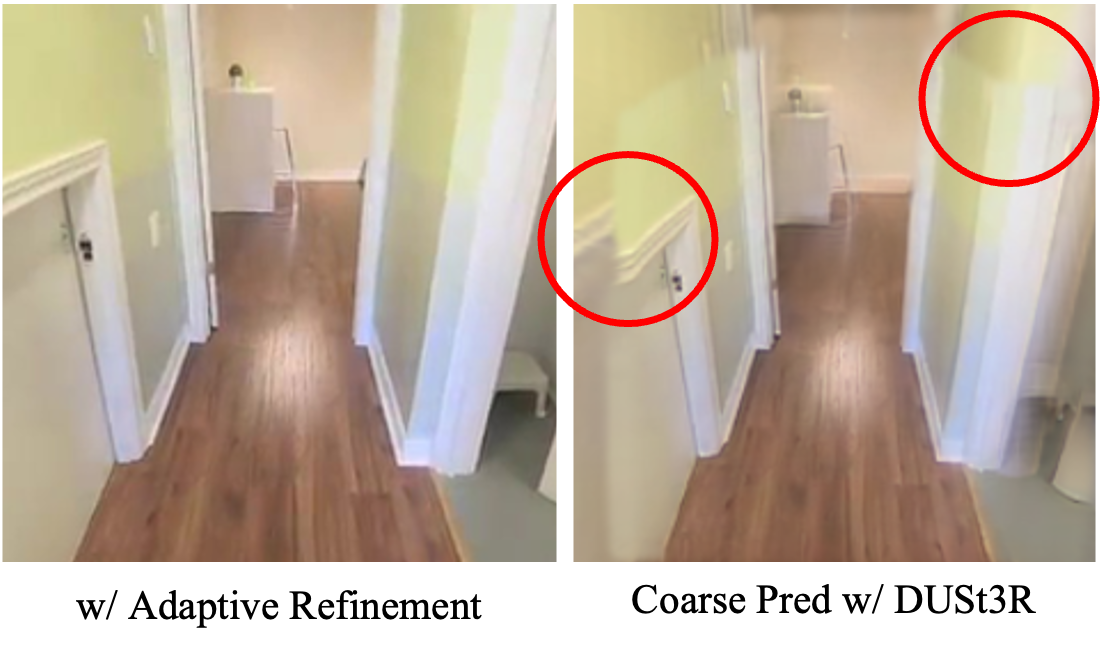}
        \caption{Robustness to texture-less region.}
        \label{fig:robustsness}
\end{figure}

\section*{Ablation Studies on Framework Design} The ADC is designed to enhance memory efficiency by reducing the number of predicted Gaussians, as illustrated in Section 3.4. The ablation study demonstrates that the ADC module prunes approximately 40\% of Gaussians with a negligible decrease in rendering quality, significantly improving the memory efficiency of StreamGS. Another navie design is directly adding GS head after DUSt3R. However, DUSt3R focuses on extracting more geometric information than rendering attributes like the SH coefficients and opacity. Our separate image encoder directly fed by images ensures the decomposition of geometry and appearance learning. Such a principle can be found at 3D Generation works like texture refinement in DreamGaussian. The effectiveness of our design is demonstrated in \cref{tab:gs_head}, comparing to the naive design. 
% We would add further analysis of MASt3R and new matching method in our future work.
\begin{table}[htbp]
\centering
\setlength{\tabcolsep}{3pt} % Adjust column separation
 % Adjust row separation

\resizebox{0.4\textwidth}{!}{
\begin{tabular}{@{}lcccccc@{}}
\toprule
 & \multicolumn{3}{c}{RE10K} & \multicolumn{3}{c}{ACID} \\ \cmidrule(lr){2-4} \cmidrule(lr){5-7} 
& PSNR $\uparrow$ & LPIPS $\downarrow$ & SSIM $\uparrow$ & PSNR $\uparrow$ & LPIPS $\downarrow$ & SSIM $\uparrow$ \\ \midrule
DUSt3R+GS Head & 17.76 & 0.30 & 0.75 & 19.61 & 0.34 & 0.70 \\
{StreamGS} & \textbf{22.42} &\textbf{ 0.17} & \textbf{0.83} & \textbf{28.50} & \textbf{0.15} & \textbf{0.84} \\
\bottomrule
\end{tabular}}
\vspace{-8pt}
\caption{Ablation on framework design.}\label{tab:gs_head}
\vspace{-1em}
\end{table}
